# Supplementary material for: Gradient-Based Neuroplastic Adaptation for Concurrent Optimization of Neuro-Fuzzy Networks
Source: arXiv:2506.21771 source file (2026-01-23)
Supplement: Supplementary file 1 [file fuzzy_logic.tex]

\section{Fuzzy Logic}\label{appendix:fuzzy_logic}
In this work, truth is modeled with \textit{fuzzy logic} \cite{fuzzy_logic} \textemdash{} a many-valued truth system that was later derived from fuzzy set theory \cite{zadeh_fuzzy_sets} with strong resemblance to Łukasiewicz logic \cite{giles1976lukasiewicz}.
%As illustrated thus far, truth \textemdash{} when dealing with vague terms or symbols, is better modeled by many-valued systems. 
%fuzzy logic \cite{fuzzy_logic} \textemdash{} originally proposed as \textit{vague logic} \cite{vague_logic}, is a type of many-valued logic similar to Łukasiewicz logic \cite{giles1976lukasiewicz}, derived from fuzzy set theory \cite{10.5555/248374}. 
In fuzzy logic, truth is a \textit{matter of degree} just as elements may belong to sets with varying \textit{degrees of membership}. This logic is beneficial when boundaries between concepts are blurred or smooth, as reality often deals with truths that involve grayness \cite{mendel_type-2_2002}. For example, ``that person is tall'' may be subjective rather than an objective truth, as people may agree to varying degrees on the statement. In other words, the statement does not need to be asserted as entirely false or true in fuzzy logic, whereas traditional binary logic expects sharp classifications (i.e., boundaries). Statements like ``the car is more maroon than it is burgundy'' can be understood by fuzzy logic despite the blurred boundary between the concepts. Similar to Łukasiewicz logic \cite{giles1976lukasiewicz}, the truthness of undecided (``possible'') is represented by $\frac{1}{2}$; more specifically, the truth value of $\frac{1}{2}$ is the moment of paradox \textemdash{} the (fuzzy) proposition is equally true as it is false \cite{kosko1992neural}. Lastly, fuzzy logic is primarily a ``distance-based'' logic interested in proximity or similarity, where it calculates the \textit{distance} to a \textit{concept} or \textit{exemplar(s)} that perfectly embodies a proposition \cite{tfig}. Other elements are compared to such exemplars to determine their similarity; the exemplars behind a proposition are its \textit{core}.

\subsection{Propositions}
A \textit{fuzzy proposition} is \emph{atomic} or \emph{compound} \cite{10.5555/248374}. For instance, an atomic fuzzy proposition has the form
\begin{equation}\label{proposition}
x \texttt{ is } {G} ,
\end{equation}
where $x$ is the value of some attribute defined over a universe of discourse ${X}$ and $G$ is a fuzzy predicate. The degree to which it is true is $G(x)$ or $\mu_{G}(x)$. %The degree to which the predicate or proposition $G$ is true is determined in exactly the same manner as fuzzy set membership. 
% The degree to which proposition $p$ is true, $\mu_{p}$, is thus
% \begin{equation}\label{relative_truth}
% \mu_{p} = \mathcal{G}(x)
% \end{equation}
% for each $x \in \mathcal{X}$ in proposition $p$.
A compound fuzzy proposition is several atomic fuzzy propositions connected using the words ``and'', ``or'', and ``not'', which are implemented using fuzzy intersection ($\wedge$), fuzzy union ($\vee$), or fuzzy complement ($\neg$), respectively.

\subsection{Conditional Statements}
\textit{Fuzzy conditional statements} that have conditional and unqualified propositions \cite{klir_yuan} are only considered here. This is because their formulation aligns with the fuzzy logic rules discussed in this paper. They can be expressed as 
\begin{equation}\label{conditional_proposition}
\texttt{If } {x} \texttt{ is } {G}_{1}, \texttt{ then } y \texttt{ is } {G}_{2}, 
\end{equation}
\noindent
where $x$ and $y$ are attributes/variables that have universal sets ${X}$ and ${Y}$, respectively. Lastly, the fuzzy sets ${G}_{1}$ and ${G}_{2}$ are defined over these universal sets. As previously stated, fuzzy conditional statements are essentially fuzzy logic rules. In this illustrative example, only a single condition and a single decision (both are primitive attributes) are considered. However, this may be extended to consider compound attributes for their conditions or decisions. For now, this is omitted for simplicity. 

\subsection{Implication}
% Let $R$ be a fuzzy relation on the Cartesian product $\mathcal{X}_{1}$ and $\mathcal{X}_{2}$. Then, its degree of associativity can be computed by
% \begin{equation}\label{fuzzy_relation}
% R(\mathcal{X}_{1}, \mathcal{X}_{2}) = \mathcal{i}[\mathcal{G}_{1}(x_{1}), \mathcal{G}_{2}(x_{2})] \; ,
% \end{equation}
% where $\mathcal{G}_{1}$ and $\mathcal{G}_{2}$ are fuzzy sets defined on $\mathcal{X}_{1}$ and $\mathcal{X}_{2}$, respectively, and $\mathcal{i}$ denotes a fuzzy implication. 

The \textit{fuzzy implication}, $\mathcal{i}$, is a binary fuzzy relation defined as
\begin{equation}\label{fuzzy_implication}
\mathcal{i} : [0, 1] \times [0, 1] \to [0, 1] .
\end{equation}
Since $\mathcal{i}$ is a binary fuzzy relation, assume it is operating on a space that is the result of a Cartesian product between universal sets ${X}$ and ${Y}$. Let ${G}_{1}$ and ${G}_{2}$ define fuzzy sets on ${X}$ and ${Y}$, respectively. Then, its degree of associativity can be computed by
\begin{equation}\label{fuzzy_relation}
\mathcal{i}\big ( {G}_{1}(x), {G}_{2}(y)\big )
\end{equation}
where $x \in X$ and $y \in Y$. Multiple implementations of fuzzy implication exist, and the choice of which implementation to use is often a design choice. However, the importance of applying generalized modus ponens, modus tollens, and hypothetical syllogisms may be considered, as not all definitions of fuzzy implication satisfy these criteria. 
% An example of a fuzzy implication that satisfies the above would be the \textit{Gaines-Rescher} implementation,
% \begin{equation}\label{gaines_rescher}
% \mathcal{i} \big({G}_{1}(x), {G}_{2}(y)\big) = \begin{cases}
% 1 & \texttt{when } {G}_{1}(x) \le {G}_{2}(y) \\
% 0 & \texttt{when } {G}_{1}(x) > {G}_{2}(y).
% \end{cases}
% \end{equation} 
% \subsubsection*{Composition}
% The \textit{compositional operator} is defined as
% \begin{equation}\label{compositional}
% z = y \circ (x \circ R)
% \end{equation}
% where $\circ$ is the sup-star compositional operator, $x$ and $y$ are provided inputs, $R$ is a fuzzy relation and $z$ is the output to infer.
