# Supplementary material for: Gradient-Based Neuroplastic Adaptation for Concurrent Optimization of Neuro-Fuzzy Networks
Source: arXiv:2506.21771 source file (2026-01-23)
Supplement: Supplementary file 2 [file fuzzy_sets.tex]

\section{Fuzzy Sets}\label{appendix:fuzzy_sets}
Traditional set theory determines an element's membership to a set, or a \textit{concept}, by arbitrarily using bivalent logic as its backbone (i.e., an element is either a member of the set or it is not), but reality seldom reflects this binary outlook; especially when modeling vague terms such as those found in natural language (e.g., the set of tall people). Instead, it is becoming increasingly apparent that membership is a matter of degree when defining concepts with natural language \cite{hagras_towards_nodate, pierrard_learning_2018, mencar_paving_2019, arrieta_explainable_2019}; in other words, an element may partially belong to a set or sets. For example, someone may be your friend and foe, but they may be your friend more than your foe. Understanding the degree to which a person is your friend or foe is a nuance often overlooked or ignored in bivalent logic. Usually, one might assume by ``foe'' we mean the complement of a friend (i.e., ``$\neg$ friend''). Due to the law of excluded middle, bivalent logic would struggle if framed in this manner, as a person can't be your friend and $\neg$ friend simultaneously. Unfortunately, life experience may reflect that someone can be a friend and a foe.

Fuzzy sets \cite{zadeh_fuzzy_sets} quantify \textit{how strongly} an element belongs to a concept (i.e., how similar an element is to an exemplar/core), or said another way, \textit{how well} the set describes the element. By determining membership degree to be multi-valued, specifically in the $[0, 1]$ range, where $0$ and $1$ remain absolute non-membership and membership, respectively, we may still model set membership while allowing some elements to belong more so than others. Again, for example, some people may be a friend (or foe) more than others (e.g., ``How good of a friend is this person, 0\% to 100\%?''); fuzzy sets retain this internal ranking. 

Fuzzy set theory is often misunderstood and mistakenly compared to probability theory. Still, they are distinct mathematical branches concerned with handling different types of uncertainty. In fact, they may complement one another \cite{zadeh_book}, as they do in this proposed method (with STGE). Fuzzy set theory deals with \textit{scoring}, \textit{ranking}, or \textit{similarity} with respect to an \textit{exemplar} (e.g., comparing students' tests to an \textit{ideal solution} such as a teacher solution). In contrast, probability tackles uncertainty due to limited information (e.g., guessing the rank and suit of the hidden playing card).
% For a fuzzy set, an element's membership is $[$typically$]$ between 0 and 1 \cite{zadeh_fuzzy_sets} \textemdash unlike ``traditional'' set theory, where an element either belongs to a set or does not. For example, a set, whether fuzzy or not, may be interpreted as a \textit{concept}, such as ``the set of tall people''. In traditional set theory, a person either completely belongs to the set of tall people, or does not. 
% Fuzzy sets allow us to quantify \textit{how strongly} a person belongs to this concept, or said another way, \textit{how well} the set describes the individual. The issue with traditional set theory and logic when applied to \textit{vague} symbols has been closely studied by figures such as Bertrand Russell, Max Black, Kurt Gödel, Jan Łukasiewicz, just to name a few.

A \textit{membership function}, $\mu$, determines an element's membership in a fuzzy set. This is analogous to an element's membership in a traditional set determined by a characteristic function. Thus, we may use the terms ``fuzzy sets'' and ``membership functions'' interchangeably throughout this paper.
