# Supplementary material for: Gradient-Based Neuroplastic Adaptation for Concurrent Optimization of Neuro-Fuzzy Networks
Source: arXiv:2506.21771 source file (2026-01-23)
Supplement: Supplementary file 3 [file hitl.tex]

\section{Potential for Human-in-the-Loop}\label{appendix:nfn_diagram}
\begin{figure}
    \centering
    \includegraphics[width=\linewidth]{appendix/figures/dissertation_nfn.png}
    \caption{A TSK NFN rearranged according to insights from \citeauthor{cui_curse_2021} \cite{cui_curse_2021}.}
    \label{fig:nfn_diagram_example}
\end{figure}
Each moment of fuzzy inference is cleanly separated into its respective layers (Figure~\ref{fig:nfn_diagram_example}). This helps a human operator diagnose and troubleshoot the NFN if needed. For example, if no fuzzy logic rules are activated strongly enough to produce an output, the human operator can check rule activation in the ``Rule Layer''. Suppose fuzzy logic rules' activations are near zero or zero. In that case, the individual may move backward to the ``Membership Layer'' to see which premises are involved in the fuzzy logic rules causing near zero or zero activation. Otherwise, if the fuzzy logic rules have sufficient activation, the individual may move through the network to check whether the Center of Area defuzzification works as intended. More specifically, perhaps all the certainty factors (CFs) have become close to zero \textemdash{} nullifying the effect of the fuzzy logic rules. They can also directly examine the fuzzy logic rules with the most potent activation, read their linguistic interpretation (if dimensionality is low enough or feature selection is somehow incorporated), and correct any ill-assigned consequence recommended by the fuzzy logic rule(s). Further, knowledge from one NFN can be sliced and inserted into another NFN by simply removing and adding the involved components the designer intends to retain. Lastly, this transparent function approximation gives us the clear semantic meaning behind gradients when checking back-propagation calculations \textemdash{} such as validating the fuzzy sets' parameters in ``Membership Layer'' are appropriately updated.
