# Supplementary material for: Gradient-Based Neuroplastic Adaptation for Concurrent Optimization of Neuro-Fuzzy Networks
Source: arXiv:2506.21771 source file (2026-01-23)
Supplement: Supplementary file 4 [file impact_and_limitations.tex]

\subsection{Broader Impact}
This strategy for the concurrent optimization of NFNs discovers rules expressed through linguistic mediums (constrained fuzzy partitions) based on original features. These rules 
% can adeptly handle stimuli with missing information and 
are easily transferable between neuro-fuzzy architectures, suggesting a substantial potential for knowledge transfer, especially in scenarios like federated learning. NFNs could also easily benefit from research addressing the interpretability challenges in ``black box'' DNNs, such as SHAP values. This integration could provide insights beyond the conventional understanding, but is likely unnecessary beyond the interpretability already provided by NFNs.

Moreover, practitioners trained on NFNs can leverage their transparent structure for diagnostics and repairs. The ability to precisely pinpoint a faulty layer opens up exciting possibilities for troubleshooting and improvement. Concurrent optimization of NFNs offers a flexible and potentially interpretable approach, with implications ranging from enhanced adaptability to applications in federated learning and insights into complex neural network behaviors.

\subsection{Limitations}
The generation of results was limited to an NVIDIA GTX 3080 GPU. 
In the experiments, we only considered selecting a fixed size of the FRB to instead focus this dissertation's contribution on the more critical component of concurrent optimization \textemdash{} rearranging the FRBs' conditions as necessary. New fuzzy logic rules may be added if the NFN's performance remains unsatisfactory and has not improved. Furthermore, unlike Chapter~\ref{chapter:fyd}, the number of conditions involved in the generated fuzzy logic rules grows linearly with respect to the input dimensionality of the NFNs. Due to the multiple variables presently involved that were investigated in the development of concurrent optimization, rule simplification was omitted from consideration to reduce the search space. However, the strategies discussed in Chapter~\ref{chapter:fyd} can be applied to the NFN at any point. This dissertation's neurogenesis can only add new fuzzy sets, not remove them. Again, this restricted scope was chosen to reduce the potential influences in this search process for concurrent optimization. The implications of rule simplification can be considered now that concurrent optimization of NFNs is feasible.

Regarding the input dimensionality issue, an altered form of dropout \cite{JMLR:v15:srivastava14a} could alleviate this. Unnecessary fuzzy sets in the membership layer could be eliminated by removing those not contributing to the fuzzy logic rules, while highly similar fuzzy sets are aggregated into more concise versions. Additionally, fuzzy logic rules could be pruned using a modified dropout technique \cite{guo_concise_2022}. These limitations and their potential solutions remain for future investigation.
