# Supplementary material for: Gradient-Based Neuroplastic Adaptation for Concurrent Optimization of Neuro-Fuzzy Networks
Source: arXiv:2506.21771 source file (2026-01-23)
Supplement: Supplementary file 5 [file morphism_concerns.tex]

\section{Challenges of Neurogenesis in Neuro-Fuzzy Networks}\label{appendix:morphism_concerns}
NFNs may encounter erroneous calculations if all fuzzy logic rules' activations are zero or near zero. This may occur if the linguistic term describing any condition attribute is not applicable enough for the given stimuli, thus decreasing the fuzzy logic rule's overall activation. In turn, the expectation is that 
%Although the proposed GBNA may help avoid sampling fuzzy logic rules with near-zero activation, it still expects that 
\textit{some} linguistic term in \textit{each} condition attribute is activated strongly enough for the given stimuli. Further, it is desirable that one or more fuzzy logic rules collectively activate strongly enough to recommend their decisions with a meaningful enough impact on the output. This assurance is referred to as $\epsilon$-completeness, and FISs/NFNs typically require it to prevent numerical underflow \cite{lee_flc_12}. %For instance, in propositional logic, there should be at least one or more rules where the compound condition attributes apply to the current state. Otherwise, no rules are applicable, and the system can recommend no reasonable decision. 

The expectation that a FIS or NFN is $\epsilon$-complete typically assumes this property is always maintained. Thus, a new fuzzy set should be added \textit{immediately} once unrecognized stimuli are first encountered (i.e., deemed novel). Adding a new fuzzy set that can be used as a condition for a fuzzy logic rule in an NFN is synonymous with neurogenesis. This new fuzzy set would capture the core of the unrecognized stimuli's signal with an appropriately determined receptive field \cite{tung_safin_2011}. However, caution should be exercised when selecting the ``receptive field'' of a new fuzzy set \textemdash{} too small will result in its rare utilization, while too large may cause it to dominate over its neighbors unnecessarily. For Gaussian fuzzy sets, this amounts to carefully choosing a value for $\sigma$. For instance, if $\sigma=1 \times 10^{-1000}$ or $1 \times 10^{+1000}$ were selected, the Gaussian fuzzy set would either rarely be activated or completely dominate, respectively, for ``most'' inputs (e.g., $[-100.0, 100.0] \subset \mathbb{R}$ if its center were $0$). This challenge may arise when the attribute of only a single observation has no matching fuzzy set, as there may not be enough information to determine a reasonable $\sigma$.

Potential problems continue even after the new fuzzy set is created, as 
it is unclear how to incorporate it into the NFN's existing FRB. 
% \textemdash{} especially in the context of concurrent optimization. 
GBNA would need to explore how to integrate this new fuzzy set, if at all, into the existing FRB. Proceeding with caution is necessary as it may lead to a subpar or more optimal compound condition attribute for some fuzzy logic rule. Suppose many new fuzzy sets are continuously added to the NFN (perhaps because $\sigma$ was poorly chosen and is too small). In that case, it can become challenging for an NFN to learn \textit{which} fuzzy sets to reference in the fuzzy logic rules, as the NFN's structure is changing too quickly, resulting in too many options.
