# Supplementary material for: Gradient-Based Neuroplastic Adaptation for Concurrent Optimization of Neuro-Fuzzy Networks
Source: arXiv:2506.21771 source file (2026-01-23)
Supplement: Supplementary file 6 [file transparency.tex]

\section{Dynamic \& Transparent Decision-Making}\label{appendix:transparency}
NFNs offer a compelling opportunity to understand decision-making in neural architectures, particularly in vision-based tasks. Figure~\ref{fig:dtc_original_resized_img} illustrates the pre-processing pipeline for a 640x480 RGB24 image from the defend the center task, resized to an 84x84 resolution (or 640x480x3 and 84x84x3 when including channel dimensions). Like other neural architectures, NFNs can leverage standard vision-based interpretation techniques such as occlusion masks, saliency maps, and integrated gradients. For instance, Figure~\ref{fig:dtc_optuna_occlusion} shows the occlusion mask obtained by the NFN as a melee-only enemy approaches the player's position. Positive attribution (green) is given to the melee-only enemy on the left side of the screen, whereas negative attribution (red) is given to the center and right side.

After resizing, the input image passes through convolutional layers (Figure~\ref{fig:dtc_after_conv}), where the resulting feature maps are directly compared against the NFN’s exemplars. %In vision-based tasks, NFN exemplars may represent either exemplary feature maps or convolved features. The output of the final convolutional layer is evaluated against these exemplars to measure how well the input stimuli align with each other.
An NFN operating on a vision-based task may represent its exemplars as exemplary feature maps (i.e., exemplary convolved features). 
The output from the final convolutional layer is evaluated against these exemplars to measure how well they align. In Figure~\ref{fig:dtc_after_conv_fuzzy_sets}, the feature map input to the NFN is identical to the one shown in Figure~\ref{fig:dtc_after_conv}, but its color scheme has been adjusted to align with the NFN's representation. Initially, the Term 1 and Term 2 exemplars represent two opposing extremes. However, the Term 2 exemplar was refined by gradient descent to capture underlying patterns better, enhancing the NFN's ability to generalize and interpret visual data.

% Fuzzy logic rules in vision-based tasks operate on exemplary feature maps, where the input feature map to the NFN is compared against these exemplars. 
Exemplars for fuzzy logic rules are created by extracting segments from the term exemplars and organizing them into meaningful patterns, as shown in Figure~\ref{fig:dtc_after_conv_fuzzy_exemplars}. The input feature map is compared to these exemplars to assess the relevance of each fuzzy logic rule, with the most similar exerting the greatest influence on the output. Thus, analysis of an NFN within a vision-based task can determine which components of the feature maps are most vital to the agent's decision-making. If CNNs were not used before the NFN, the resized image from Figure~\ref{fig:dtc_original_resized_img} could be fed directly into the NFN. In this case, each fuzzy logic rule's compound condition attribute would correspond to an exemplary 84x84 RGB24 image, against which incoming images would be compared. This presents intriguing opportunities for interpretation and offers an alternative approach to understanding the policy's decision-making that is not readily available with traditional DNNs.

\begin{figure*}[ht]
    \centering
    \begin{tabular}{cc}
        \textit{(1) Original Image} & \textit{(2) Resized Image} \\
        \includegraphics[width = 0.48\linewidth]{appendix/figures/Interpretation/original.png} &
        \includegraphics[width = 0.48\linewidth]{appendix/figures/Interpretation/resized.png} 
    \end{tabular}
    % \textbf{Target Tracking \& Trajectory Prediction}
    \caption{An input image before (left) and after (right) resizing.}
    \label{fig:dtc_original_resized_img}
\end{figure*}

\begin{figure}[ht]
    \centering
    \includegraphics[width=\linewidth]{appendix/figures/Interpretation/optuna/occlusion.png}
    \caption{Occlusion masks from positive/negative attribution can be used with NFNs.}
    \label{fig:dtc_optuna_occlusion}
\end{figure}

\begin{figure*}[ht]
    \centering
    \begin{tabular}{cc}
        \textit{(1) After Convolutional Layer 1} & \textit{(2) After Convolutional Layer 2} \\
        \includegraphics[width = 0.48\linewidth]{appendix/figures/Interpretation/after_conv/1.png} &
        \includegraphics[width = 0.48\linewidth]{appendix/figures/Interpretation/after_conv/2.png} \\
        \textit{(3) After Convolutional Layer 3} & \textit{(4) After Convolutional Layer 4} \\
        \includegraphics[width = 0.48\linewidth]{appendix/figures/Interpretation/after_conv/3.png} &
        \includegraphics[width = 0.48\linewidth]{appendix/figures/Interpretation/after_conv/4.png} 
    \end{tabular}
    % \textbf{Target Tracking \& Trajectory Prediction}
    % \caption{(1) An original input image before resizing in the DTC task. (2) After the resizing.}
    \caption{Illustration of how the image in Figure~\ref{fig:dtc_original_resized_img} progresses through each convolutional layer, where high-level features are extracted from the feature maps at the initial stages.}
    \label{fig:dtc_after_conv}
\end{figure*}

\begin{figure*}[ht]
    \centering
    \begin{tabular}{ccc}
        \textit{After Convolutional Layer 4} & \textit{Term 1 Exemplar} & \textit{Term 1 Membership} \\
        \includegraphics[width = 0.3\linewidth]{appendix/figures/Interpretation/after_conv/4_matching.png} &
        \includegraphics[width = 0.3\linewidth]{appendix/figures/Interpretation/mu/center_0_exemplar.png} &
        \includegraphics[width = 0.3\linewidth]{appendix/figures/Interpretation/mu/center_0_mu.png} \\
        & \textit{Term 2 Exemplar} & \textit{Term 2 Membership} \\
        &
        \includegraphics[width = 0.3\linewidth]{appendix/figures/Interpretation/mu/center_1_exemplar.png} &
        \includegraphics[width = 0.3\linewidth]{appendix/figures/Interpretation/mu/center_1_mu.png} 
    \end{tabular}
    % \textbf{Target Tracking \& Trajectory Prediction}
    % \caption{(1) An original input image before resizing in the DTC task. (2) After the resizing.}
    \caption{Exemplary convolved features' membership is based on the last convolutional layer's output.}
    \label{fig:dtc_after_conv_fuzzy_sets}
\end{figure*}

\begin{figure*}[ht]
    \centering
    \begin{tabular}{ccc}
        & \textit{Rule 3 Exemplar} & \textit{Rule 3 Membership} \\
        & \includegraphics[width = 0.3\linewidth]{appendix/figures/Interpretation/mu/rule_3_exemplar.png} &
        \includegraphics[width = 0.3\linewidth]{appendix/figures/Interpretation/mu/rule_3_mu.png} \\
        \textit{After Convolutional Layer 4} & \textit{Rule 43 Exemplar} & \textit{Rule 43 Membership} \\
        \includegraphics[width = 0.3\linewidth]{appendix/figures/Interpretation/after_conv/4_matching.png} &
        \includegraphics[width = 0.3\linewidth]{appendix/figures/Interpretation/mu/rule_43_exemplar.png} &
        \includegraphics[width = 0.3\linewidth]{appendix/figures/Interpretation/mu/rule_43_mu.png} \\
        & \textit{Rule 90 Exemplar} & \textit{Rule 90 Membership} \\
        &
        \includegraphics[width = 0.3\linewidth]{appendix/figures/Interpretation/mu/rule_90_exemplar.png} &
        \includegraphics[width = 0.3\linewidth]{appendix/figures/Interpretation/mu/rule_90_mu.png} 
    \end{tabular}
    % \textbf{Target Tracking \& Trajectory Prediction}
    % \caption{(1) An original input image before resizing in the DTC task. (2) After the resizing.}
    \caption{Relevance of each fuzzy logic rule is determined by comparing their exemplary convolved feature map to the output from the last convolutional layer.}
    \label{fig:dtc_after_conv_fuzzy_exemplars}
\end{figure*}
