# Supplementary material for: Gradient-Based Neuroplastic Adaptation for Concurrent Optimization of Neuro-Fuzzy Networks
Source: arXiv:2506.21771 source file (2026-01-23)
Supplement: Supplementary file 7 [file computational_tricks.tex]

\section{Presence of Softmax in Takagi-Sugeno-Kang Neuro-Fuzzy Networks}\label{appendix:computational_tricks}

This paper will only consider TSK NFNs with Gaussian fuzzy sets and product inference engine (Eq.~\ref{eq:mamdani_fuzzy_system:coa_defuzzifier}) as the computational trick that is about to be used requires it. Let $U$ denote the set of unique universal identifiers for fuzzy logic rules. A TSK NFN with Gaussian fuzzy sets and a product inference engine is defined as

\begin{equation}
\label{eq:tsk_fuzzy_system:coa_defuzzifier}
    \mathfrak{F}_{\text{TSK}}(\mathbf{x}) = \frac{ 
    \sum\limits_{u \in U} \mathcal{g}_{u}(\mathbf{x})     
    % w_{u}
    \big (
    \prod\limits_{i \in I_{\mathcal{C}}} 
    \mathcal{m}_{u}(i)(x_{i}) 
    \big )
    }{ 
    \sum\limits_{u \in U}
    % w_{u}
    \big (
    \prod\limits_{i \in I_{\mathcal{C}}} 
    \mathcal{m}_{u}(i)(x_{i}) 
    \big )
    }
\end{equation}
\noindent
such that the relevance of each fuzzy logic rule $u \in U$ is determined by 
% $\Big (
% \prod\limits_{i \in I_{\mathcal{C}}} 
% \exp \big (-\frac{({x}_{i} - {c}_{i, j})^2}{2\sigma_{i, j}^2} \big )
% \Big )$.
$\prod\limits_{i \in I_{\mathcal{C}}} 
\mathcal{m}_{u}(i)(x_{i})$, and each $\mathcal{m}_{u}(i)$ retrieves a Gaussian membership function, $\mu_{i, j}$, defined according to 	\begin{equation}\label{eq:mf:gaussian}
	\mu_{\textit{gaussian}}(x, c, \sigma) = \exp \Bigg (- \frac{(x - c)^{2}}{2{\sigma}^{2}} \Bigg)
\end{equation}
\text{where $c$ represents the center and $\sigma$ is the width.} 
For convenience, let $\mu_{i, j, u}$ refer to this $\mathcal{m}_{u}(i)$; similarly, its corresponding center and width may be referenced by $c_{i, j, u}$ and $\sigma_{i, j, u}$, respectively. Expanding upon Eq.~\ref{eq:tsk_fuzzy_system:coa_defuzzifier} yields 
\begin{equation}
\label{eq:tsk_fuzzy_system:coa_defuzzifier_expanded}
    \mathfrak{F}_{\text{TSK}}(\mathbf{x}) = \frac{ 
    \sum\limits_{u \in U} \mathcal{g}_{u}(\mathbf{x})     
    % w_{u}
    \Big (
    \prod\limits_{i \in I_{\mathcal{C}}} 
    \exp \big (-\frac{({x}_{i} - {c}_{i, j, u})^2}{2\sigma_{i, j, u}^2} \big )
    \Big )
    }{ 
    \sum\limits_{u \in U}
    % w_{u}
    \Big (
    \prod\limits_{i \in I_{\mathcal{C}}} 
    \exp \big (-\frac{({x}_{i} - {c}_{i, j, u})^2}{2\sigma_{i, j, u}^2} \big )
    \Big )
    }
\end{equation}
and is equivalent to
\begin{equation}
\label{eq:tsk_fuzzy_system:coa_defuzzifier_expanded_equiv}
    \mathfrak{F}_{\text{TSK}}(\mathbf{x}) = \frac{ 
    \sum\limits_{u \in U} \mathcal{g}_{u}(\mathbf{x})     
    % w_{u}
    \Big (
    \exp \big ( - \sum\limits_{i \in I_{\mathcal{C}}} 
    \frac{({x}_{i} - {c}_{i, j, u})^2}{2\sigma_{i, j, u}^2} \big )
    \Big )
    }{ 
    \sum\limits_{u \in U}
    % w_{u}
    \Big (
    \exp \big ( - \sum\limits_{i \in I_{\mathcal{C}}} 
    \frac{({x}_{i} - {c}_{i, j, u})^2}{2\sigma_{i, j, u}^2} \big )
    \Big )
    }
\end{equation}

\noindent
which may be rearranged as 

\begin{minipage}{0.475\linewidth}
    \begin{equation}
    \label{eq:nfn_coa}
    \mathfrak{F}_{\text{TSK}}(\mathbf{x}) = \sum\limits_{u \in U} \mathcal{g}_{u}(\mathbf{x}) \overline{w}_{u}(\mathbf{x})
    % NFN(\mathbf{x}) = \sum_{k' = 1}^{|\mathcal{R}|} {\mu}_{\mathcal{S}, k'}(\mathbf{x})\mu_{\mathcal{Q}, k'}(\mathbf{q})
    \end{equation}
\end{minipage}\hfill
\begin{minipage}{0.475\linewidth}
    % \begin{equation}
    %     \mathfrak{F}(\mathbf{x}) = \sum\limits_{u \in U} \mathcal{g}_{u}(\mathbf{x}) \overline{w}_{u}
    % \end{equation}

    \begin{equation}\label{eq:softmax}
    \overline{w}_{u}(\mathbf{x}) = \frac{\exp \big (
    {w}_{u}(\mathbf{x})
    \big)
    }{\sum\limits_{u \in U} \exp \big({w}_{u}(\mathbf{x})\big)}
    \end{equation}
\end{minipage}
\noindent
where $w_{u}(\mathbf{x})$ is the (preliminary) weight, or activation, of fuzzy logic rule $\mathcal{f}_{u}$ such that
\begin{equation}
    \label{eq:mu_rule_sum}
    w_{u}(\mathbf{x}) = - \sum\limits_{i \in I_{\mathcal{C}}} 
    \frac{({x}_{i} - {c}_{i, j, u})^2}{2\sigma_{i, j, u}^2} .
\end{equation}
Observe Eq.~\ref{eq:softmax} is \texttt{softmax}; numeric underflow can be avoided with a common trick \cite{cui_curse_2021}

\begin{equation}\label{eq:norm_softmax}
\overline{w}_{u}(\mathbf{x}) = \frac{\exp \big (
{w}_{u}(\mathbf{x}) - \max{w}_{u}(\mathbf{x})
\big)
}{\sum_{u}^{U} \exp \big({w}_{u}(\mathbf{x}) - \max{w}_{u}(\mathbf{x}) \big)}
\end{equation}
where $\max {w}_{u} = \max\limits_{u \in U} {w}_{u}$.
