# Supplementary material for: Gradient-Based Neuroplastic Adaptation for Concurrent Optimization of Neuro-Fuzzy Networks
Source: arXiv:2506.21771 source file (2026-01-23)
Supplement: Supplementary file 8 [file neuro_fuzzy.tex]

\section{Neuro-Fuzzy Networks}\label{appendix:nfn}
Appendix~\ref{appendix:fuzzy_inference_system} introduced the mathematics of how fuzzy reasoning may be defined, but does not address its inefficiency. In particular, the previous formulas are intended to calculate the output of a FIS for a single observation and consult each fuzzy logic rule sequentially rather than simultaneously. One significant advantage of DNNs to FIS (or at least this perspective) is their capability to handle simultaneous inputs, sometimes referred to as a \textit{batch of data}, by leveraging matrix operations to use computer hardware more efficiently. A FIS with a connectionist representation may easily replicate this computational efficiency. 

In addition to computational efficiency, DNNs have also enjoyed widespread success and adaptation thanks to the relative ease of applying them to learn complex tasks when given sufficient data and network complexity (e.g., number of hidden layers/neurons, reasonable selection of their activation functions). On the contrary, the structure as well as parameters of a FIS are often assumed to be static, and each component must be explicitly designed. Therefore, it would be logical and natural to want to extend FISs with this same learning ability to remove the dependency on meticulously designing their components. 

% \subsection{Neuro-Fuzzy Networks}
In the early 1990s, fuzzy modeling research into adaptive FISs led to significant breakthroughs. One such example is the proposal of a general neural-network (connectionist) model by \citeauthor{lin_neural-network-based_1991} for adaptive FISs, such that the resulting model could benefit from FISs'
interpretability and neural networks' adaptability \cite{lin_neural-network-based_1991}. 
Multiple interpretations of adaptive FISs in a neural network-like representation exist, such as \citeauthor{KELLER19921}'s proposed three variations of a neural network structure capable of fuzzy logic inference \cite{KELLER19921}. 
These architectures were among the earliest examples of neuro-fuzzy networks (NFNs), offering a parallelizable implementation of FISs for improved computational efficiency. 

Their connection to neural networks also enabled parameter tuning by adjusting fuzzy set definitions based on the NFN's performance relative to a given objective function. By representing a FIS in this manner, the parameters (and later the structure, as proposed in this paper) of the FIS may be fine-tuned with gradient descent. Thus, an objective of this connectionist representation is to be efficient and remain differentiable. Most NFN implementations can only achieve differentiability of the parameters, further highlighting the novelty and potential impact of this paper, as our proposed changes allow concurrent optimization of parameters and structure. 
Overall, NFNs differ from conventional DNNs as they allow both explicit and implicit knowledge to be utilized. In contrast, DNNs typically can only use implicit knowledge extrapolated from large amounts of data.

On a high level, an NFN is a sparsely connected neural network where weights between the layers are restricted to binary values. Non-standard activation functions will be used to implement the previously introduced FIS process. An important note is that NFNs should not be confused with \textit{fuzzy neural networks (FNNs)}, which typically refer to neural networks with fuzzy signals and/or fuzzy weights \cite{buckley_fuzzy_1994, buckley_neural_1995}. This ambiguity in terminology likely arose due to early disagreements among researchers, leading to confusion in the field. In this paper, the term ``FNN'' refers to a connectionist representation of a FIS, not a neural network with fuzzy signals or weights. Therefore, the term ``NFN'' will be used whenever possible to ensure clarity and consistency, while ``FNN'' will be retained when referencing the original author's terminology to align with the overall literature. For example, the family of pseudo outer-product based FNNs (POPFNNs) is technically a subcategory of NFNs. Despite their name, they are \textit{not} neural networks with fuzzy signals and/or fuzzy weights.

\subsection{Fundamental Principles}
Since an NFN is a computationally efficient representation of a FIS, and a FIS may correspond to a decision table $\mathfrak{T} = (U, \mathcal{A}, \mathcal{C}, \mathcal{D})$, the following discussion will leverage this preexisting notation. Let $U$ uniquely identify each fuzzy logic rule, and $\mathcal{C}$ as well as $\mathcal{D}$ continue to reference condition and decision attributes, respectively, such that $\mathcal{A} = \mathcal{C} \cup \mathcal{D}$. 
An NFN almost always has only five layers; these layers correspond directly to an individual step in FIS inference. Quantitative fuzzy variables will be considered linguistic variables for ease of reference, and a batch size of 1 is assumed unless specified otherwise for simplicity. 

\subsection{Describing the Input with Linguistic Terms}
The first layer is simple if only singleton fuzzification (Eq.~\ref{eq:fuzzy_logic:singleton_fuzzification}) is used: input stimuli, $\mathbf{x}$, is simply passed through to the rest of the NFN. If imprecise or inaccurate inputs were to be expected, this could be factored in by modifying it to include a fuzzification process. The focus of this paper is not on fuzzification, so for simplicity, only a singleton fuzzification process will be used throughout. The second layer contains the linguistic terms that describe the input space (i.e., $\bigcup_{i \in I_{\mathcal{C}}} \mathcal{M}_{i}$). Edges from the first layer to the second layer \textit{only} exist with a value of $1$ if and only if the linguistic term applies to that linguistic variable. To clarify, $x_{i}$ for $i \in I_{\mathcal{C}}$ would only be connected to each $\mu_{i, j}$ from its associated fuzzy sets, $\mathcal{M}_{i}$. %, where $j$ indexes the $i^{\text{th}}$ attribute's linguistic terms, $\mathcal{M}_{i}$. 
The second layer's output is the collection of all memberships to all linguistic terms across the linguistic variables for condition attributes $\mathcal{C}$, and may be represented as a matrix:

\begin{equation}
\label{eq:nfn:membership_matrix}
    \boldsymbol{\mu}_{\mathcal{C}}(\mathbf{x}) = \begin{bmatrix} 
    \mu_{1, 1}(x_{1}) & \mu_{1, 2}(x_{1}) & \dots \\
    \vdots & \ddots & \\
    \mu_{|\mathcal{C}|, 1}(x_{|\mathcal{C}|}) &        & \mu_{|\mathcal{C}|, \max_{i \in I_{\mathcal{C}}}(|\mathcal{M}_{i}|)}(x_{|\mathcal{C}|}) 
    \end{bmatrix}
    \qquad
\end{equation}
where $|\mathcal{C}|$ is the count of condition attributes. In the event some $\mu_{i, j}({x}_{i})$ does not exist for the index pair $(i, j)$, then a special flag (e.g., \texttt{NaN}, -1) may be placed to occupy the location in the meantime. If a batch of inputs, $\mathbf{X}$, was simultaneously considered where $I_{\mathbf{X}}$ is the discrete index set of each observation, then the \textit{batch membership matrix} is calculated as 
\begin{equation}
\label{eq:nfn:batch_membership_matrix}
    \boldsymbol{\mu}_{\mathcal{C}}(\mathbf{X}) = \begin{bmatrix} 
    \boldsymbol{\mu}_{\mathcal{C}}(\mathbf{x}_{1}) \\
    \vdots \\
    \boldsymbol{\mu}_{\mathcal{C}}(\mathbf{x}_{|\mathbf{X}|})
    \end{bmatrix}
    \qquad
\end{equation}
such that the shape of $\boldsymbol{\mu}_{\mathcal{C}}(\mathbf{X})$ is $\max(I_{\mathbf{X}}) \times |\mathcal{C}| \times \max_{i \in I_{\mathcal{C}}}(|\mathcal{M}_{i}|)$. An accompanying \textit{membership mask}, $\mathbf{M}$, of shape $|\mathcal{C}| \times \max_{i \in I_{\mathcal{C}}}(|\mathcal{M}_{i}|)$ may exist if necessary which contains a $1$ if and only if a linguistic term exists at entry $i, j$, else, it is $0$. Non-existing memberships are dropped by Hadamard product (element-wise multiplication, $\odot$) %between the membership matrix, $\boldsymbol{\mu}_{\mathcal{C}}(\mathbf{s})$, and its mask, $B$, 
such that $\boldsymbol{\mu}_{\mathcal{C}}(\mathbf{x}) \odot \mathbf{M}$. Caution should be observed as a membership degree of $0$ in $\boldsymbol{\mu}_{\mathcal{C}}(\mathbf{x}) \odot \mathbf{M}$ may then either indicate the associated linguistic term is false or non-existent. However, if this distinction is necessary, referring back to $\mathbf{M}$ to discern the difference is certainly possible, but the purpose of this is for computational efficiency. The membership mask will become more relevant in later sections. Still, it exists to help facilitate batch operations using contiguous memory.\footnote{Note that using a membership mask is an implementation detail we found necessary when writing this paper, but could be removed if such matters are handled differently. In particular, handling special flags, such as \texttt{NaN} or -1, can become particularly problematic when using automatic differentiation engines. Thus, we opted for a dedicated membership mask in code implementations of NFNs to avoid such issues.}

\subsection{Activating the Fuzzy Logic Rules}
The third layer hosts the fuzzy logic rules, and the inputs provided to it are from Eq.~\ref{eq:nfn:membership_matrix} or Eq.~\ref{eq:nfn:batch_membership_matrix} if considering a batch of inputs. However, similar to the second layer, they operate only on their respective linguistic variables and terms involved in the conditions. As a result, edges are assigned a value of $1$ between all relevant (fuzzy) condition propositions, while all other connections are set to $0$. 
If the product inference engine with singleton fuzzification (Eq.~\ref{eq:fuzzy_logic:singleton_fuzzification}) and Center of Area defuzzification (Eq.~\ref{eq:coa_defuzzifier}) is to be implemented by the NFN (i.e., Eq.~\ref{eq:mamdani_fuzzy_system:coa_defuzzifier}), then each node in this layer calculates $\big (\prod\limits_{i \in I_{\mathcal{C}}} \mathcal{m}_{u}(i)(x_{i}) \big )$ from Eq.~\ref{eq:mamdani_fuzzy_system:coa_defuzzifier} for all $u \in U$. The nodes' outputs correspond to the activation of each fuzzy logic rule in the FRB regarding the compound condition attributes applicability to input $\mathbf{x}$, or $\mathbf{X}$ if it is a batch. 

\subsection{Determining the Output}
The fourth layer receives the degree to which each fuzzy logic rule is activated and connects it with the consequences it recommends; again, these connections, if they exist, are $1$, and $0$ otherwise. The fifth and final layer implements defuzzification. For simplicity, the remainder of this discussion will assume Eq.~\ref{eq:mamdani_fuzzy_system:coa_defuzzifier} is the type of FIS to be implemented, in which case, this layer directly corresponds to calculating the rest of the formula from Eq.~\ref{eq:mamdani_fuzzy_system:coa_defuzzifier}. If the fuzzy logic rules are of the Mamdani style, then each output linguistic node provides its recommendation to form $\mathbf{d}_{u}$; otherwise, they are assumed to be TSK in which case they would provide $\mathcal{g}_{u}$ and then calculate $\mathcal{g}_{u}(\mathbf{x})$ or $\mathcal{g}_{u}(\mathbf{X})$. These recommendations are then weighed by each fuzzy logic rule's activation or applicability to the input stimuli and summed over the fuzzy logic rule dimension (i.e., $    \sum_{u \in U} \mathbf{d}_{u}     
% w_{u}
\big (
\prod_{i \in I_{\mathcal{C}}} 
\mathcal{m}_{u}(i)(x_{i}) 
\big )$). The prior summation will be referred to as \textit{the numerator}. As previously discussed, the Center of Gravity Defuzzifier is approximated by the Center of Area Defuzzifier. To mimic this goal of obtaining the Center of Gravity, the numerator may be divided by \textit{a denominator}. This denominator is simply the sum over the fuzzy logic rules' activations: $    \sum_{u \in U}
% w_{u}
\big (
\prod_{i \in I_{\mathcal{C}}} 
\mathcal{m}_{u}(i)(x_{i}) 
\big )$. To complete the Center of Area defuzzification, the numerator is divided by the denominator as shown in Eq.~\ref{eq:mamdani_fuzzy_system:coa_defuzzifier}. NFNs in this paper will follow the above implementation.
